# Supplementary material for: Sparse Mixture-of-Experts are Domain Generalizable Learners
Source: arXiv:2206.04046 source file (2023-01-27)
Supplement: Supplementary file 1 [file public_resources.tex]

\section{Public Resources}
\label{sec:public_resource}
We acknowledge the use of the following public resources, during the course of this work:
\begin{itemize}
    \item nuScenes\footnote{\url{https://www.nuscenes.org/nuscenes}} \dotfill CC BY-NC-SA 4.0
    \item nuScenes-devkit\footnote{\url{https://github.com/nutonomy/nuscenes-devkit}} \dotfill Apache License 2.0
    \item SemanticKITTI\footnote{\url{http://semantic-kitti.org}} \dotfill CC BY-NC-SA 4.0
    \item SemanticKITTI-API\footnote{\url{https://github.com/PRBonn/semantic-kitti-api}} \dotfill MIT License
    \item ScribbleKITTI\footnote{\url{https://github.com/ouenal/scribblekitti}} \dotfill Unknown
    \item FIDNet\footnote{\url{https://github.com/placeforyiming/IROS21-FIDNet-SemanticKITTI}} \dotfill Unknown
    \item Cylinder3D\footnote{\url{https://github.com/xinge008/Cylinder3D}} \dotfill Apache License 2.0
    \item TorchSemiSeg\footnote{\url{https://github.com/charlesCXK/TorchSemiSeg}} \dotfill MIT License
    \item MixUp\footnote{\url{https://github.com/facebookresearch/mixup-cifar10}} \dotfill Attribution-NonCommercial 4.0 International
    \item CutMix\footnote{\url{https://github.com/clovaai/CutMix-PyTorch}} \dotfill MIT License
    \item CutMix-Seg\footnote{\url{https://github.com/Britefury/cutmix-semisup-seg}} \dotfill MIT License
    \item CBST\footnote{\url{https://github.com/yzou2/CBST}} \dotfill Attribution-NonCommercial 4.0 International
    \item MeanTeacher\footnote{\url{https://github.com/CuriousAI/mean-teacher}} \dotfill Attribution-NonCommercial 4.0 International
\end{itemize}
